# Supplementary material for: Learning an unknown transformation via a genetic approach
Source: arXiv:1610.03291 ancillary file (2016-10-11)
Supplement: Supplementary file 1 [file tomography_SI_arXiv.pdf]

# Supplemental Material - Learning an unknown transformation via a genetic approach

Nicolò Spagnolo,<sup>1,\*</sup> Enrico Maiorino,<sup>1</sup> Chiara Vitelli,<sup>1</sup> Marco Bentivegna,<sup>1</sup> Andrea Crespi,<sup>2,3</sup>  
 Roberta Ramponi,<sup>2,3</sup> Paolo Mataloni,<sup>1</sup> Roberto Osellame,<sup>2,3</sup> and Fabio Sciarrino<sup>1,†</sup>

<sup>1</sup>*Dipartimento di Fisica, Sapienza Università di Roma, Piazzale Aldo Moro 5, I-00185 Roma, Italy*

<sup>2</sup>*Istituto di Fotonica e Nanotecnologie, Consiglio Nazionale delle Ricerche (IFN-CNR), Piazza Leonardo da Vinci, 32, I-20133 Milano, Italy*

<sup>3</sup>*Dipartimento di Fisica, Politecnico di Milano, Piazza Leonardo da Vinci, 32, I-20133 Milano, Italy*

## I. THE ALGORITHM

The  $m \times m$  interferometer is injected with single photon and two-photon input states to obtain the starting data sets. From single photon measurements the input/output interferometer couplings  $\tilde{\mathcal{P}}_{i,j}$  are obtained (with corresponding errors  $\Delta\tilde{\mathcal{P}}_{i,j}$ ), while two-photon measurements give rise to  $h = \binom{m}{2}^2$  possible Hong-Ou-Mandel interference patterns, quantified by the corresponding dip (or peak) visibilities  $\tilde{\mathcal{V}}_{ij,pq}$  with errors  $\Delta\tilde{\mathcal{V}}_{ij,pq}$ .

The genetic algorithm, which aims at learning the unitary transformation  $\mathcal{U}_r$  starting from the collected data set, is structured as follows.

1. A distribution of  $N$  DNA sequences, representing  $N$  different  $m \times m$  unitary matrices, is generated. The parameters  $\{t_k^l, \alpha_k^l, \beta_k^l\}$  are drawn from appropriate distributions, so that the generated unitaries are distributed according to the Haar measure [1]. An approximate form of these distributions have been evaluated numerically by sampling unitary matrices from the Haar measure. More specifically, the phase differences  $\alpha_k^l - \beta_k^l$  are drawn from the uniform distribution, while the transmittivities  $t_k^l$  are drawn from a triangular one  $u(t_i) = 2t_i$ . The exact form of these distribution can be evaluated as shown in [2]. The obtained set of  $N$  DNAs constitutes the population  $\tilde{\Phi}_0 = \{\tilde{E}_1, \dots, \tilde{E}_N\}$ .
- 1'. The analytic method proposed in Ref. [3] is applied to the experimental data. A set of  $m^2$  independent estimates of the unitary [4] is obtained, starting from this approach, by selecting appropriate subsets of the data and by performing permutations of the mode indexes. DNA sequences for the  $s_1 = 20$  unitaries presenting higher fitnesses are then evaluated. Finally,  $s_1$  elements of the population  $\tilde{\Phi}_0$  obtained at step 1 are replaced by the  $s_1$  candidates determined from the analytic method. The new set of  $N$  DNAs constitutes the initial population  $\Phi_0 = \{E_1, \dots, E_N\}$ .
2. The population is sorted by decreasing fitness values, evaluated between the experimental data  $(\tilde{\mathcal{P}}_{i,j}, \tilde{\mathcal{V}}_{ij,pq})$  and the predictions  $(\mathcal{P}_{i,j}^{E_l}, \mathcal{V}_{ij,pq}^{E_l})$  obtained from the matrices of the population, with  $l = 1, \dots, N$ . The new ordered population set is  $\Phi_1 = \{E'_1, \dots, E'_N\}$ .
3. The single-photon probabilities  $\mathcal{P}^{E'_1}$  and the two-photon visibilities  $\mathcal{V}^{E'_1}$  are calculated from the element  $E'_1$ . If  $f(E'_1) \geq \delta$  the algorithm halts and returns the solution matrix  $U_{E'_1}$ . More specifically, the unitary matrix  $U_{E'_1}$  is obtained from the conversion function  $T(E'_1)$  which relates the genetic code to the corresponding unitary transformation [5].
4. The second half of the population, consisting of the individuals with lowest fitness values, is removed. The resized population  $\Phi_2$  is the set  $\Phi_2 = \{E'_1, \dots, E'_{N/2}\}$ .
5. Crossover is applied between two randomly chosen individuals. The corresponding generated offspring is added to the population set  $\Phi_2$ . This operation is iterated with other couples of individuals until the number of elements of  $\Phi_2$  is  $N$ . The result of this mechanism is a new population  $\Phi_3 = \{E'_1, \dots, E'_{N/2}, \bar{E}_{N/2+1}, \dots, \bar{E}_N\}$ , where the elements  $\bar{E}_l$  are the newly-generated individuals.
6. During the evolution of the system, several individuals with the identical DNA (clones) corresponding to the element with highest fitness may spread in the population. This effect causes a steady depletion of the gene pool, which in turn leads to an early convergence of the algorithm to a local maximum of  $f(E)$ . To avoid this effect two countermeasures have been adopted: (i) **Random Offspring Generation** [6], which imposes that crossover between two clones generates a child with random DNA, and (ii) **Packing**, which consists in identifying clusters of clones in the population every  $q$  iteration. For each of these clusters, all the elements except one are removed and the population is filled by randomly generated new individuals.

\* nicolo.spagnolo@uniroma1.it

† fabio.sciarrino@uniroma1.it

7. For each element  $l = 2, \dots, N$ , mutation is applied with probability  $\gamma$ . The index  $l$  starts from the value 2 to avoid a mutation on the individual with highest fitness in the population. This constraint is commonly referred to as *Elitism*. A new population  $\Phi_4 = \{E''_1, \dots, E''_N\}$  is obtained.
8. Steps 2-7 are iterated starting from the new population  $\Phi_4$  until the halting condition is reached at step 3.

## II. EXPERIMENTAL DETAILS

Single-photon and two-photon input states, necessary to measure the starting data set for the algorithm, are prepared by a spontaneous parametric down-conversion source. The 750 mW pump beam at  $\lambda_P = 392.5$  nm is obtained by second-harmonic generation of a  $\lambda = 785$  nm pulsed Ti:Sa laser source, with 76 MHz repetition rate and  $\Delta\tau = 250$  fs pulse duration. The photon source is a type-II, 2 mm length BBO crystal (Beta-Barium Borate), which generated pairs of photons with opposite polarization. Photons after generation are spectrally selected by 3 nm interference filters, analyzed in polarization, collected in single-mode fibers, and then propagated through two independent delay lines to perform temporal synchronization. Then, after fiber polarization compensation, the generated photons are injected in the input modes of the interferometer through a single-mode fiber array, and are then collected by a multi-mode fiber array before detection with a set of single-photon avalanche photodiodes (APD). Output single photon counts and two-fold coincidences are collected by an electronic acquisition system. The overall set of collected experimental data, composed by  $d_1 = 49$  single-photon probabilities and  $d_2 = 441$  two-photon visibilities, is reported in Fig. S1.

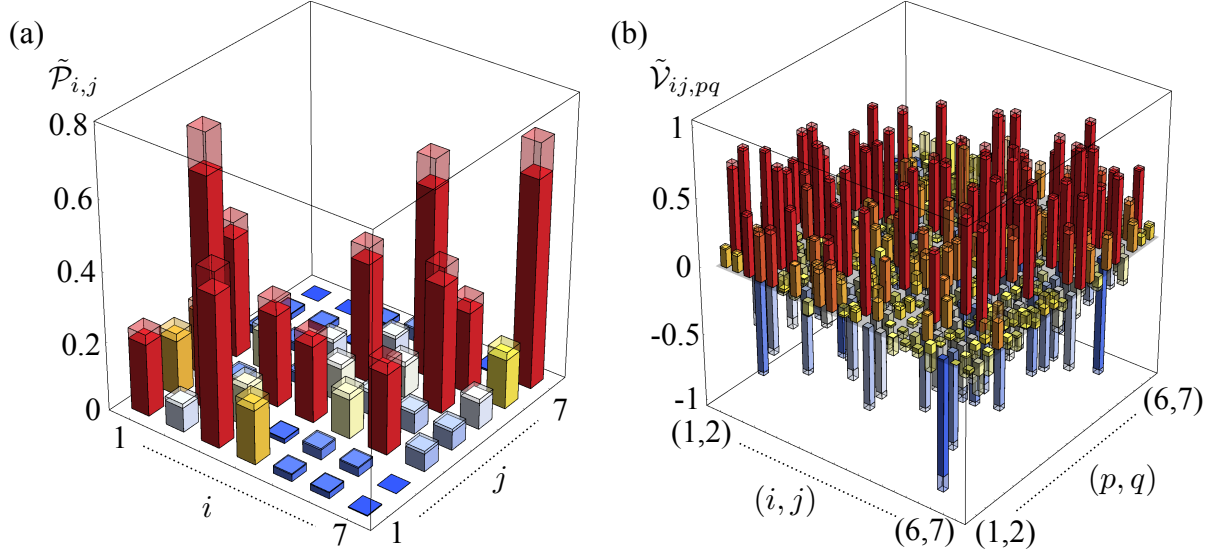

Supplementary Figure S1. (a) Measured single-photon probabilities  $\tilde{P}_{i,j}$ . (b) Measured two-photon Hong-Ou-Mandel visibilities  $\tilde{V}_{ij,pq}$ . Shaded regions correspond to the experimental errors.

## III. EXPECTED AND RECONSTRUCTED UNITARY MATRICES

Here we report the unitary matrix corresponding to the interferometer design  $\mathcal{U}_t$  and the one obtained from the reconstruction with the genetic approach  $\mathcal{U}_r^{(g)}$ .

The expected unitary  $\mathcal{U}_t$  has real part:

$$\Re[\mathcal{U}_t] = \begin{pmatrix} 0.440067 & -0.144084 & -0.213019 & 0.478544 & 0.148792 & 0.0954517 & 0. \\ -0.0824973 & -0.483843 & -0.113649 & 0.0270831 & -0.0954517 & 0.148792 & 0. \\ -0.0668478 & 0.0540365 & 0.520786 & 0.257786 & -0.168401 & -0.0722028 & 0.159266 \\ 0.59962 & 0.362828 & -0.192912 & -0.408267 & -0.295213 & -0.137872 & 0.192703 \\ -0.171234 & 0.0439199 & -0.252021 & 0.211038 & -0.173805 & -0.344251 & -0.0907635 \\ -0.0439199 & -0.171234 & 0.0840009 & -0.104909 & 0.1454 & -0.320468 & 0.217302 \\ 0. & 0. & -0.0825909 & -0.235963 & -0.45092 & 0.131444 & -0.533947 \end{pmatrix} \quad (\text{S1})$$

and imaginary part:

$$\Im[\mathcal{U}_t] = \begin{pmatrix} -0.0460727 & -0.257413 & -0.605506 & 0.116951 & -0.0954517 & 0.148792 & 0. \\ 0.555327 & -0.531634 & 0.302887 & 0.0133133 & -0.148792 & -0.0954517 & 0. \\ -0.247407 & -0.332066 & -0.0992346 & -0.391134 & -0.136487 & -0.453793 & 0.192703 \\ -0.0360857 & -0.298176 & 0.126105 & -0.0298965 & -0.14752 & -0.0865235 & -0.159266 \\ 0.0439199 & 0.171234 & -0.0760492 & 0.458373 & -0.22598 & -0.600826 & -0.211058 \\ -0.171234 & 0.0439199 & 0.101443 & 0.203086 & -0.689667 & 0.31566 & 0.348654 \\ 0. & 0. & -0.235963 & 0.0825909 & -0.0146029 & -0.0272751 & 0.606908 \end{pmatrix} \quad (S2)$$

The reconstructed unitary matrix  $\mathcal{U}_r^{(g)}$  with the genetic approach has real part:

$$\Re[\mathcal{U}_r^{(g)}] = \begin{pmatrix} 0.4355 & -0.1775 & -0.1611 & 0.3850 & 0.1002 & 0.04614 & -0.01467 \\ -0.08493 & -0.5299 & -0.1084 & 0.07069 & -0.08722 & 0.09845 & -0.004452 \\ -0.09533 & 0.02920 & 0.4440 & 0.3112 & -0.2021 & -0.07885 & 0.1113 \\ 0.6582 & 0.3075 & -0.1640 & -0.3307 & -0.2972 & -0.2983 & 0.1659 \\ -0.1592 & -0.02603 & -0.2743 & 0.1996 & -0.1505 & -0.2898 & -0.08246 \\ -0.07511 & -0.1536 & 0.005676 & -0.06572 & 0.2152 & -0.3605 & 0.2140 \\ -0.008678 & -0.00004971 & -0.07865 & -0.2236 & -0.4224 & 0.05521 & -0.5920 \end{pmatrix} \quad (S3)$$

and imaginary part:

$$\Im[\mathcal{U}_r^{(g)}] = \begin{pmatrix} -0.04560 & -0.1994 & -0.7269 & 0.05497 & 0.002889 & 0.1366 & -0.01895 \\ 0.3917 & -0.6540 & 0.2609 & -0.0613 & -0.09862 & -0.1233 & -0.001719 \\ -0.4036 & -0.1589 & -0.08890 & -0.3718 & -0.1918 & -0.4876 & 0.1664 \\ 0.0001499 & -0.2371 & 0.1527 & -0.09482 & -0.1162 & -0.1312 & -0.1089 \\ 0.01891 & 0.1362 & -0.05465 & 0.5653 & -0.0433 & -0.5648 & -0.2884 \\ -0.1041 & 0.02457 & 0.01568 & 0.2373 & -0.7350 & 0.2596 & 0.2622 \\ 0.008239 & -0.000001997 & -0.1609 & 0.1284 & -0.06000 & -0.02719 & 0.6042 \end{pmatrix} \quad (S4)$$

- 
- [1] C. Spengler, M. Huber, and B. C. Hiesmayr, *Journal of Mathematical Physics* **53**, 013501 (2012).  
[2] N. J. Russell, J. L. O'Brien, and A. Laing, *ArXiv:1506.06220* (2015).  
[3] A. Laing and J. L. O'Brien, *arXiv:1208.2868v1* (2012).  
[4] A. Crespi, R. Osellame, R. Ramponi, D. J. Brod, E. F. Galvao, N. Spagnolo, C. Vitelli, E. Maiorino, P. Mataloni, and F. Sciarrino, *Nature Photonics* **7**, 545 (2013).  
[5] M. Reck, A. Zeilinger, H. J. Bernstein, and P. Bertani, *Phys. Rev. Lett.* **73**, 58 (1994).  
[6] M. Rocha and J. Neves, in *Multiple Approaches to Intelligent Systems*, edited by Springer (1999) pp. 127–136.
